# Supplementary material for: SDN Architecture and Southbound APIs for IPv6 Segment Routing Enabled Wide Area Networks
Source: arXiv:1810.06008 source file (2018-10-14)
Supplement: Supplementary file 1 [file appendix_a.tex]

\appendices

\section{Other results}
\label{sec:appendix_a}
